# Supplementary material for: Large Language Model in Medical Informatics: Direct Classification and Enhanced Text Representations for Automatic ICD Coding
Source: arXiv:2411.06823 source file (2024-11-11)
Supplement: Supplementary file 1 [file appendix.tex]

\section{Appendix}
\label{sec:app}

\begin{table}[h]
\centering
\begin{tabular}{ll}
\hline
\textbf{Hyperparameter}                & \textbf{Value}    \\ \hline
Number of Training Epochs (Top-50 codes)            & 5
\\
Number of Training Epochs (Full codes)             & 3
\\
Learning Rate Scheduler Type           & Cosine            \\
Warmup Ratio                           & 0.03              \\
Maximum Gradient Norm                  & 0.3               \\
Learning Rate                          & 1e-4              \\
Use BF16 Precision                     & True              \\
Gradient Checkpointing                 & True              \\
Gradient Accumulation Steps            & 32                \\
Per-device Training Batch Size         & 2                 \\
Per-device Evaluation Batch Size       & 2
\\
Adam Beta2                             & 0.99              \\
Weight Decay                           & 0.0               \\
\hline
\end{tabular}
\caption{The hyperparameters used in fine-tuning LLAMA classifier}
\label{table:hyperparameters1}
\end{table}

\begin{table}[h]
\centering
\begin{tabular}{ll}
\hline
\textbf{Hyperparameter}                & \textbf{Value}    \\ \hline
Number of Training Epochs (Top-50 codes)            & 15
\\
Number of Training Epochs (Full codes)             & 25
\\
Patience level & 3
\\
Learning Rate                          & 1e-4                \\
Per-device Training Batch Size         & 2 
\\
Per-device Evaluation Batch Size         & 2 
\\
\hline
\end{tabular}
\caption{The hyperparameters used in fine-tuning MultiResCNN classifier}
\label{table:hyperparameters2}
\end{table}
